# Supplementary material for: From Pairwise to Ranking: Climbing the Ladder to Ideal Collaborative Filtering with Pseudo-Ranking
Source: arXiv:2412.18168 source file (2024-12-24)
Supplement: Supplementary file 1 [file 7.appendix.tex]

\clearpage
\appendix
\section{Relationship between Ranking Loss Function and Traditional Loss Functions}
\label{app:relation}
The softmax cross-entropy loss treats the optimization of the retrieval model as a classification problem. We use $x$ to denote $\log(\sum_{w=1,w \neq v}^k \exp(s_u(\pi_{u}(w))))$ The relationship between ranking loss and softmax cross-entropy loss is derived as follows:
\begin{align}
    \mathcal{L}_{rank} &= \sum_{v=1}^{k} \max(\max_{w \neq v}\{s_u(\pi_{u}(w))\} - s_u(\pi_{u}(v)), 0) \\
    &\approx \sum_{v=1}^{k} max(x-s_u(\pi_{u}(v)),0) \\
    &\approx \sum_{v=1}^{k} \log(1 + \exp(x-s_u(\pi_{u}(v)))) \\
    & = \sum_{v=1}^{k} \log (1 + \frac{\sum_{w=1,w \neq v}^k \exp(s_u(\pi_{u}(w)))}{\exp(s_u(\pi_{u}(v)))}) \\
    & = \sum_{v=1}^{k} \log \frac{\sum_{w=1}^k \exp(s_u(\pi_{u}(w)))}{\exp(s_u(\pi_{u}(v)))}\\
    & = -\sum_{v=1}^{k} \log \frac{\exp(s_u(\pi_{u}(v)))}{\sum_{w=1}^k \exp(s_u(\pi_{u}(w)))} \\
    & = \sum_{v=1}^{k}\mathcal{L}_{softmax}.
\end{align}
In this derivation, we use the $\operatorname{LogSumExp}$ to approximate the $\max$ function. It can be seen that softmax cross-entropy loss is a special case of ranking loss, which does not utilize the known position information in the ranking and only uses the longest sub-ranking for training. Essentially, the softmax cross-entropy loss treats the optimization of the retrieval model as a classification problem. While this is effective, it overlooks the ordinal nature of ranking. If we reduce the multi-class classification problem to binary classification (positive and negative), we can derive the form of binary cross-entropy, which will not be elaborated here.

\section{Mini Batch Training}
\label{app:mini}
To integrate PRP seamlessly with many mainstream collaborative filtering models that use mini-batch training, we detail how PRP can be trained using a mini-batch style. Commonly, models sample $B$ $(u,i_p)$ interactions to form a batch. In our approach, we randomly sample $k-1$ items from the batch to form a set $M$ along with $i_p$. The set $\mathcal{P}$ is obtained after perturbing $i_p$. For the confidence mechanism, we compute all gradients within the same batch.

\section{Complexity Analysis}
\subsection{Space Complexity}
\label{app:comp}
In terms of space complexity, we only need to store the MLP modules and ranking results used in the ranker, which we will not elaborate on here. We focus on the time complexity analysis and compare it with related representative methods.
\subsection{Time Complexity}
Let $T_1$ denotes the operation time for score computation. The ranker first calculates the scores for $k$ items, taking $kT_1$, then ranks them in $O(k \log k)$ time, and similarly for the generated set $\mathcal{P}$, which takes $|\mathcal{P}|T_1 + |\mathcal{P}| \log |\mathcal{P}|$. In the ranking loss function, score calculation and ranking are already completed. Assuming the sub-ranking loss calculation time is $T_2$, the total time is $kT_2$. Thus, the time complexity is $O((k + |\mathcal{P}|)T_1 + kT_2)$. Traditional methods like BPR have a time complexity of $T_1 + T_2$. Given that the value of $k + |\mathcal{P}|$ is not excessively large, our time complexity remains acceptable.

\section{Detailed Experimental Settings}
\label{app:exp}
\begin{table}[t]
\caption{The statistics of the datasets used in the experiments.}
\begin{center}
\begin{tabular}{@{}lccccc@{}}
\toprule
\textbf{Dataset} & \textbf{Users} & \textbf{Items} & \textbf{Interactions} & \textbf{Sparsity}\\ \midrule
ML-1M & 6,041 & 3,707 & 1,000,209 & 95.53\%\\ 
Yelp & 31,669 & 38,049 & 1,561,406 & 99.87\% \\ 
Gowalla & 29,859 & 40,982 & 1,027,370 & 99.92\% \\
Foursquare & 1,084 &38,334 & 91,024 & 99.78\%\\
\bottomrule
\end{tabular}
\label{tab:statistics}
\end{center}
\vspace{-3mm}
\end{table}
\textbf{Datasets}. 
Table~\ref{tab:statistics} summarizes the statistics of the datasets. These datasets have different statistical properties, which can reliably validate the performance of a model~\cite{CCC22}. We split the data into 80\% for training, 10\% for testing, and 10\% for validation. 

\textbf{Experimental Setup}. The experiments are conducted on an NVIDIA Ampere A100-40G GPU using the RecBole v1.1.1 framework~\cite{ZMH21}. We use embeddings of size 64, initialized with Xavier's method for all models. Optimization is performed using Adam with a learning rate of 0.001, and the $L_2$ regularization coefficient is set to $10^{-4}$. We evaluate PRP's performance by varying $\beta$ within the range $[0, 1]$ and $k$ within $\{1, 2, \ldots, 10\}$. $\theta = \{0,0.01,0.1\}$. We meticulously tune all hyperparameters on the validation datasets and report the best performance for each model.

\textbf{Evaluation Protocols}. We evaluate performance using standard metrics for top-K recommendations, including Normalized Discounted Cumulative Gain (NDCG@K), Hit Rate (HR@K), and Recall (Recall@K). Our results are based on the average of five independent runs, and we conduct statistical significance analysis by calculating $p$-values against the best-performing baseline.

\textbf{Baselines}. We compare PRP with several representative state-of-the-art methods. Following conventional settings~\cite{RFG12, WYZ17, CLJ22}, we consider MF~\cite{HLZ17} as the basic model for the following methods:
\begin{itemize}
    \item \textbf{SimpleX}~\cite{MZW21}, which extracts massive high-information samples to serve as negative samples and uses cosine similarity for ranking.
    \item \textbf{UIB}~\cite{ZZY22}, which introduces a personalized boundary to penalize samples crossing the threshold.
    \item \textbf{SRNS}~\cite{DQY20}, which selects hard negative samples while incorporating a variance mechanism to filter out false negative samples.
    \item \textbf{MixGCF}~\cite{HDD21}, which leverages information from positive samples and graph neighborhood samples to synthesize negative samples.
    \item \textbf{ANS}~\cite{ZCL23}, which proposes to generate negative samples based on fine-granular factors.
\end{itemize}

To validate the effectiveness and applicability of our method, we integrate PRP with various mainstream CF models.
\begin{itemize}
    \item \textbf{MF}~\cite{RFG12}, which is the most representative matrix factorization model.
    \item \textbf{NGCF}~\cite{WHW19}, which is a pioneering work to employ the graph neural network to CF.
    \item \textbf{LightGCN}~\cite{HDW20}, which is the most popular graph neural network CF model. It eliminates the redundant components from NGCF to improve performance. 
\end{itemize}
From Table~\ref{tab:with}, it can be observed that all base models show significant performance improvements. Notably, the experimental results indicate that even a simple MF model, with PRP, can achieve performance comparable to sophisticated graph neural network models. These findings confirm the superiority and applicability of our proposed PRP solution.
